# Supplementary material for: Neural Architecture Search Over a Graph Search Space
Source: arXiv:1812.10666 source file (2019-07-31)
Supplement: Supplementary file 1 [file appendix.tex]

% \newpage
% \appendix
% \section*{Training details on Cifar10 image experiments}
% \label{app:image}

% The search space includes the following operations and options:

% \begin{itemize}
% 	\small	
% 	 \setlength\itemsep{0em}
% 	\item The controller consists of a 1 layer LSTM with 100 hidden layers. It is trained with REINFORCE with learning rate 0.0001 and entropy regularization 0.8. The initial weights of the controller are uniformly between -0.001 and 0.001.
% 	\item Convolutional ops $ConvOp$: regular conv (conv2d), depthwise conv (dconv), and mobile inverted bottleneck conv.
% 	\item Convolutional kernel size $KernelSize$: 3x3, 5x5.
% \item Skip ops $SkipOp$:  pooling, identity residual, or no skip.
% 	\item Output filter size $F_i$: 1, 2, 4, 8, 16.
% 	\item Number of layers per block $N_i$.
% 	\item Maximum number of layers per child model is 6.
% \end{itemize}
